# Supplementary material for: A Method for Constraint Inference Using Pose and Wrench Measurements
Source: arXiv:2010.15916 source file (2020-10-29)
Supplement: Supplementary file 1 [file appendix_fit_error.tex]

\section{Evaluation of fit error}\label{app:expfiterror}
Each fit was evaluated against either a) the \textbf{entire} recorded demonstration or b) an independent demonstration recorded with the experimenter. The demonstration used to evaluate the fit is referred to as the \emph{ground truth demonstration}. 
The independent ground truth demonstration was used for the \emph{point-on-plane} and \emph{point-on-line} constraint models because in some user demonstrations, the entire demonstration's data was insufficient to fit the constraint model to the true constraint and would resulted in degenerate fits.  
A limitation of the the ground truth demonstration is that it may incorporate an error of up to 1 cm due to the inability to accurately reproduce the configuration of the constraint during ground truth recording. 

An error of 1 cm is expected for the \emph{relaxed constraint} models since the pose of the constraint is measured using the tongs and the tongs grasp gradually slips during the course of the entire demonstration. 
All other models are tracked using an independent motion capture frame which has an advertised accuracy of a millimeter. 

Fit error plots for Fig. \ref{fig:highdofs} and Fig. \ref{fig:lowdofs} are generated by aggregating results from all 144 demonstrations (9 demonstrators X 2 demonstrations per constraint X 8 constraint models). Each demonstrator performs two 10 second demonstrations of each constraint type. Participants were instructed to interact with the constraint without violating the constraint (e.g. not lifting the planar constraint object off of the plane). The \emph{point on plane} and constraints requires orientation information to fit the constraint models appropriately. Participants were instructed to move their wrist more during these constraint interactions. 

Multiple demonstration lengths are selected from the demonstration and evaluated against all the samples of the ground truth demonstration.  
5 randomly sampled contiguous segments from each demonstration are selected per segment length. The length of segments are logarithmicly spaced from 2 to 256 samples. The mean fit error and first standard deviation are reported where the line indicates the mean and the shaded area indicates the bounds on the first standard deviation. 
The fit error for each fit is calculated using the position error metric computed using equation (\ref{eq:kerrormetricr}). The average of the per sample error (across the whole ground truth demonstration) is used to compute an individual fit error.
