# Supplementary material for: A Method for Constraint Inference Using Pose and Wrench Measurements
Source: arXiv:2010.15916 source file (2020-10-29)
Supplement: Supplementary file 2 [file appendix_expparams.tex]

\section{Experimental Parameters}\label{app:expparams}
\begin{table}[H]\label{table:MSthresh}
\centering
\begin{tabular}{|l|l|}
\hline
\textbf{Threshold}   & \textbf{Value}  \\ \hline
Position    & 2 mm     \\ \hline
Orientation & 2 deg         \\ \hline
Force       & 0.06 (2)      \\ \hline
Moment      & 0.06 (2)      \\ \hline
Null Hypothesis Max \% & 0.75    \\ \hline
\end{tabular}
\caption{Threshold values for error tallying}
\end{table}
